# Supplementary material for: Testing of information condensation in a model reverberating spiking neural network
Source: arXiv:1012.0490 ancillary file (2011-01-10)
Supplement: Supplementary file 1 [file movie.pdf]

**Vidybida A.K.**

**Testing of information condensation in a model  
reverberating spiking neural network**

supplementary material  
use adobe acrobat to see animation

<http://arxiv.org/abs/1012.0490>

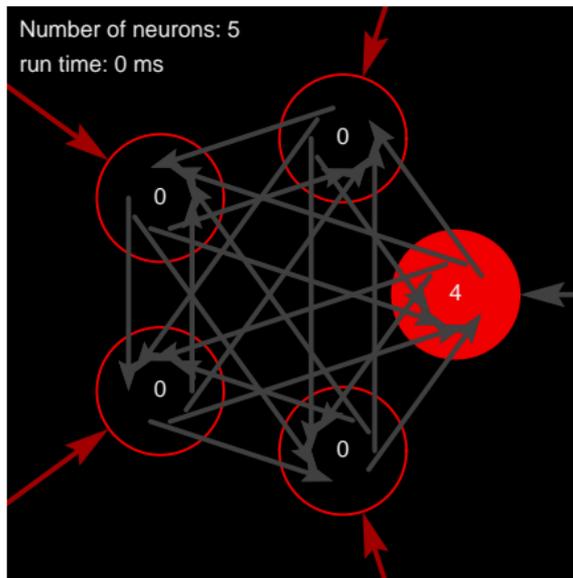

Establishing periodic dynamics in network #9  
input: {0.2, 3.0, 3.0, 3.0, 3.0} ms,  
the shortest period, 5.0 ms, relaxation time = 5.2 ms.

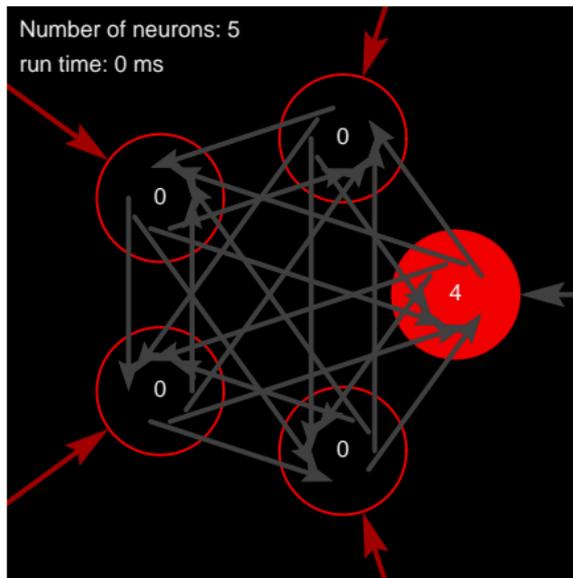

Establishing periodic dynamics in network #9  
input: {0.2, 6.2, 7.6, 4.8, 7.6} ms,  
the longest period, 16.4 ms, relaxation time = 8.4 ms.

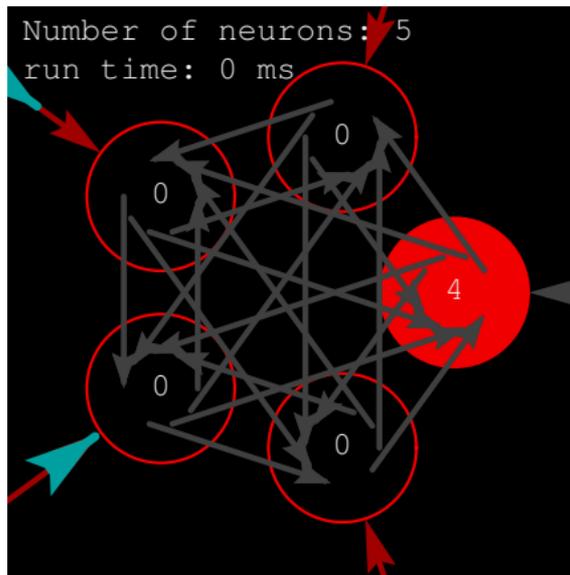

Fading out dynamics in network #19  
input: {0.2, 6.0, 2.4, 0.4, 6.4} ms,  
relaxation time = 47.4 ms.

## Credits

Prepared with animfig package by Kevin Pulo

<http://www.cs.usyd.edu.au/~kev/animfig/>
